# Supplementary material for: Diverse tunable dynamics of two quantum random walkers
Source: arXiv:1909.08527 ancillary file (2019-09-17)
Supplement: Supplementary file 1 [file Supplementary.pdf]

# Supplementary material for

# "Diverse tunable dynamics of two quantum random walkers"

Shrabanti Dhar

Department of Physics, Gokhale Memorial Girls College, 1/1 Harish Mukherjee Road, Kolkata 700020, India and Department of Physics, Aliah University, II-A/27, Newtown, Kolkata-700160, India.

Abdul Khaleque

Department of Physics, Bidhan Chandra College, Hooghly-712248, India

Tushar Kanti Bose

Department of Theoretical Physics, Indian Association for the Cultivation of Science, Kolkata 700032, India

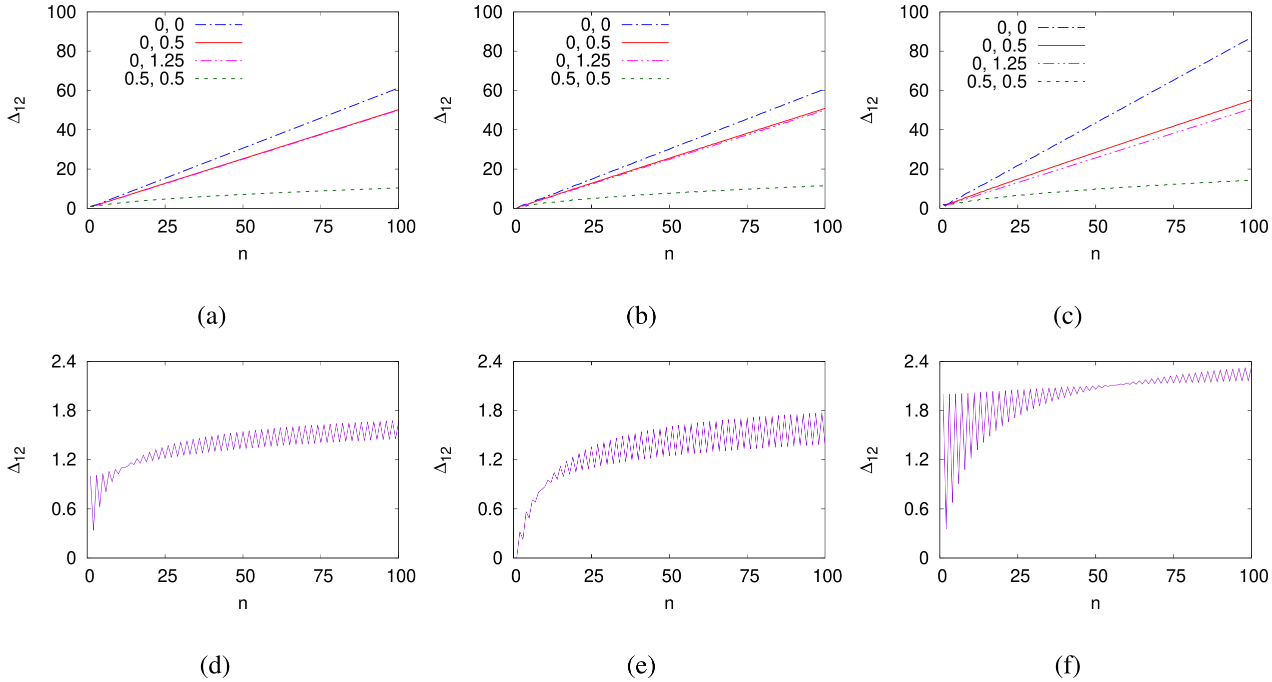


FIG. 1. Variations of the average separation $\Delta_{12}$ against dimensionless time $n$ (step number) for two non interacting walkers. (a) Variations of $\Delta_{12}$ for two walkers starting from $|Sep\rangle$ initial state for different parameter combinations $(\alpha_1, \alpha_2)$. (b) Variations of $\Delta_{12}$ for two walkers starting from $|\psi^+\rangle$ initial state for different parameter combinations $(\alpha_1, \alpha_2)$. (c) Variations of $\Delta_{12}$ for two walkers starting from $|\psi^-\rangle$ initial state for different parameter combinations $(\alpha_1, \alpha_2)$. (d) Variations of $\Delta_{12}$ for two walkers starting from $|Sep\rangle$ initial state with $\alpha_1 = \alpha_2 = 1.25$. (e) Variations of $\Delta_{12}$ for two walkers starting from $|\psi^+\rangle$ initial state with $\alpha_1 = \alpha_2 = 1.25$ (f) Variations of $\Delta_{12}$ for two walkers starting from $|\psi^-\rangle$ initial state with $\alpha_1 = \alpha_2 = 1.25$

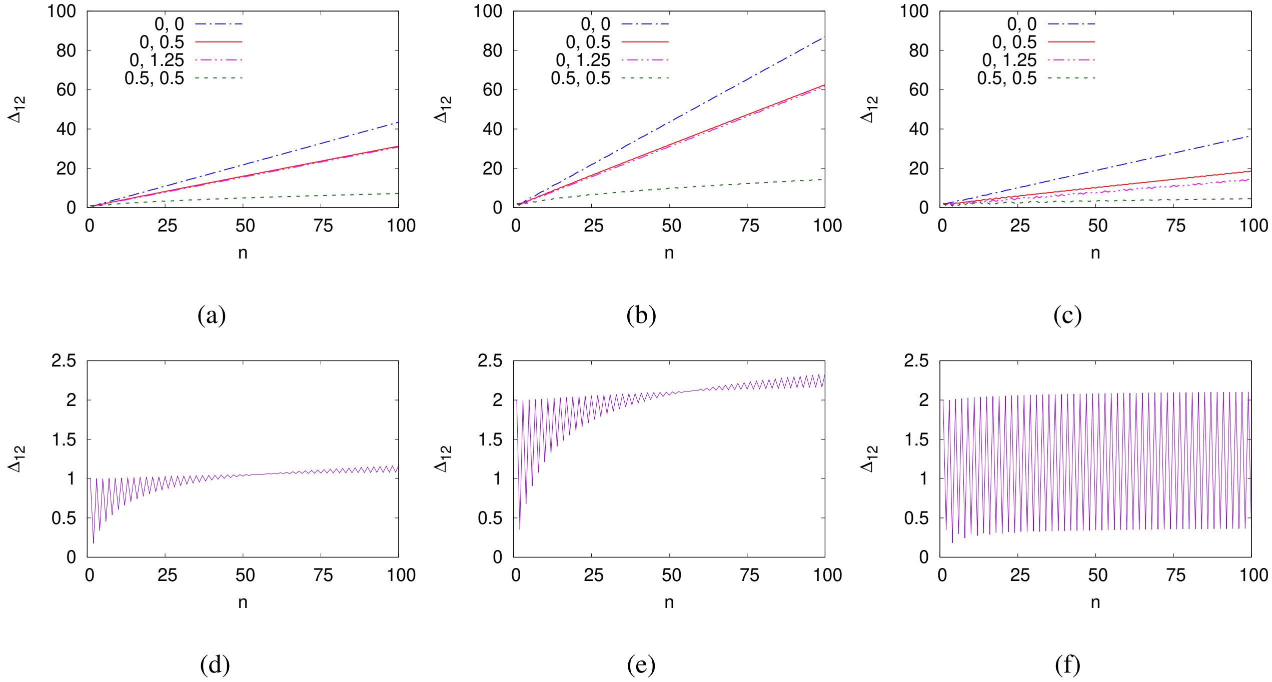


FIG. 2. Variations of the average separation $\Delta_{12}$ against dimensionless time $n$ (step number) for two one-interacting walkers. (a) Variations of $\Delta_{12}$ for two walkers starting from $|Sep\rangle$ initial state for different parameter combinations $(\alpha_1, \alpha_2)$. (b) Variations of $\Delta_{12}$ for two walkers starting from $|\psi^+\rangle$ initial state for different parameter combinations $(\alpha_1, \alpha_2)$. (c) Variations of $\Delta_{12}$ for two walkers starting from $|\psi^-\rangle$ initial state for different parameter combinations $(\alpha_1, \alpha_2)$. (d) Variations of $\Delta_{12}$ for two walkers starting from $|Sep\rangle$ initial state with $\alpha_1 = \alpha_2 = 1.25$. (e) Variations of $\Delta_{12}$ for two walkers starting from $|\psi^+\rangle$ initial state with $\alpha_1 = \alpha_2 = 1.25$ (f) Variations of $\Delta_{12}$ for two walkers starting from $|\psi^-\rangle$ initial state with $\alpha_1 = \alpha_2 = 1.25$

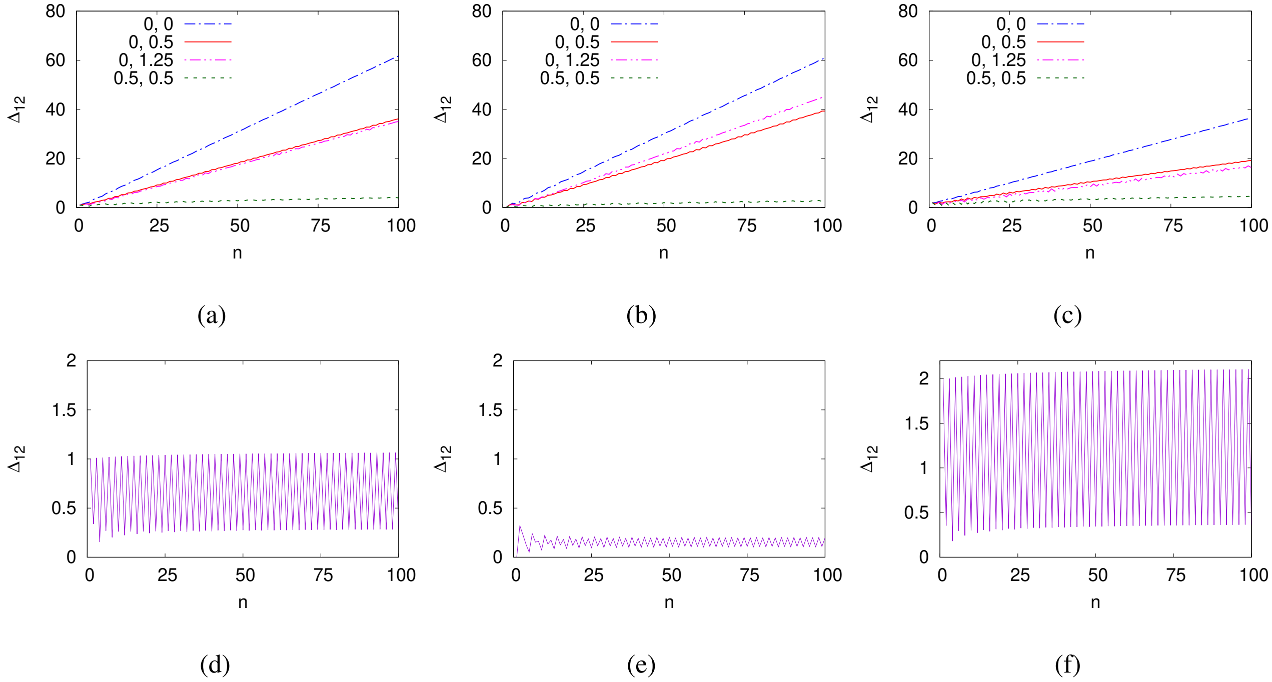


FIG. 3. Variations of the average separation $\Delta_{12}$ against dimensionless time $n$ (step number) for two pi-phase interacting walkers. (a) Variations of $\Delta_{12}$ for two walkers starting from $|Sep\rangle$ initial state for different parameter combinations $(\alpha_1, \alpha_2)$. (b) Variations of $\Delta_{12}$ for two walkers starting from $|\psi^+\rangle$ initial state for different parameter combinations $(\alpha_1, \alpha_2)$. (c) Variations of $\Delta_{12}$ for two walkers starting from $|\psi^-\rangle$ initial state for different parameter combinations $(\alpha_1, \alpha_2)$. (d) Variations of $\Delta_{12}$ for two walkers starting from $|Sep\rangle$ initial state with $\alpha_1 = \alpha_2 = 1.25$. (e) Variations of $\Delta_{12}$ for two walkers starting from $|\psi^+\rangle$ initial state with $\alpha_1 = \alpha_2 = 1.25$ (f) Variations of $\Delta_{12}$ for two walkers starting from $|\psi^-\rangle$ initial state with $\alpha_1 = \alpha_2 = 1.25$

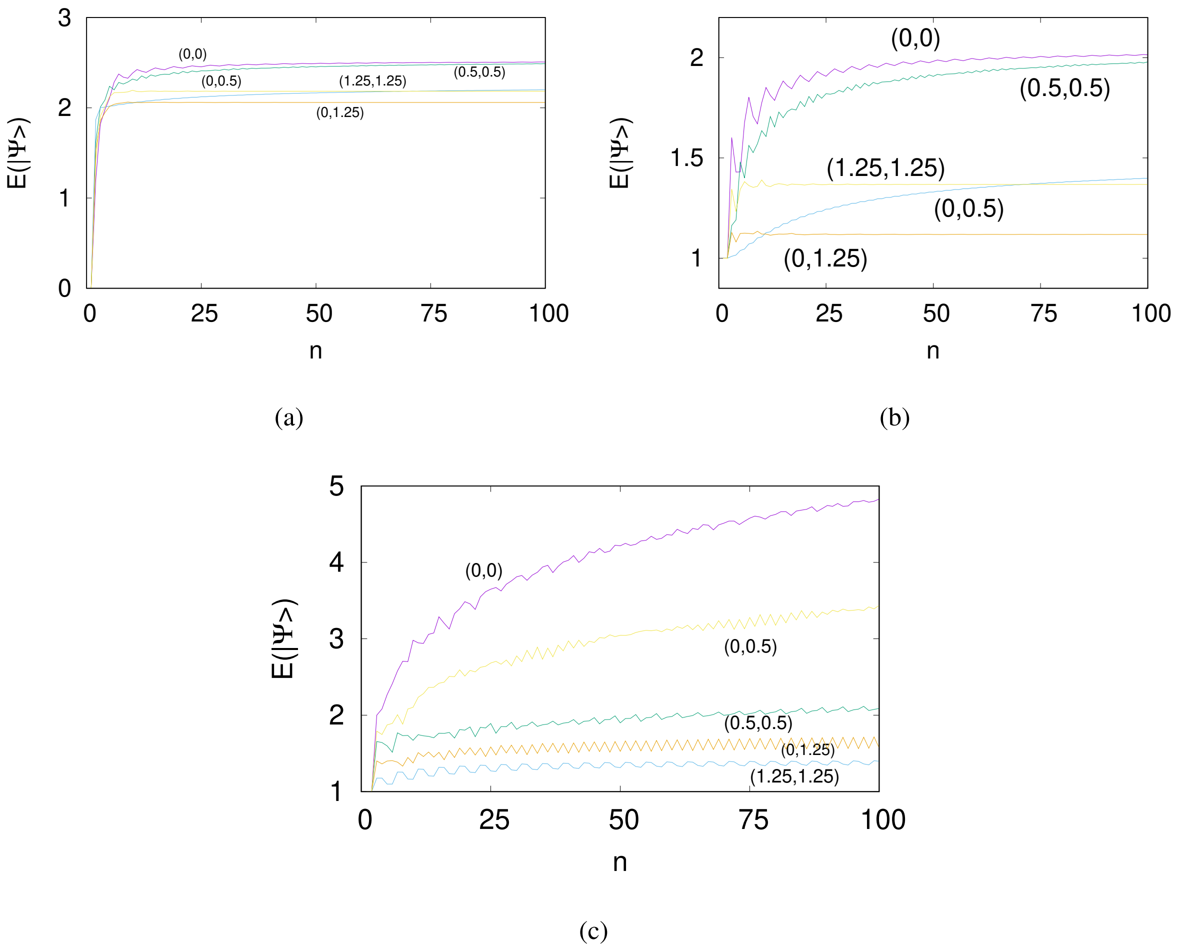


FIG. 4. Variation of bi-partite entanglement $E(|\psi\rangle)$ against dimension less time $n$ (step number) for two one interacting walkers starting from : (a) $|Sep\rangle$ state, (b) $|\psi^{+}\rangle$ state, (c) $|\psi^{-}\rangle$ state. In each figure, different curves have been drawn for different $(\alpha_1, \alpha_2)$ combinations as shown inside the figures.

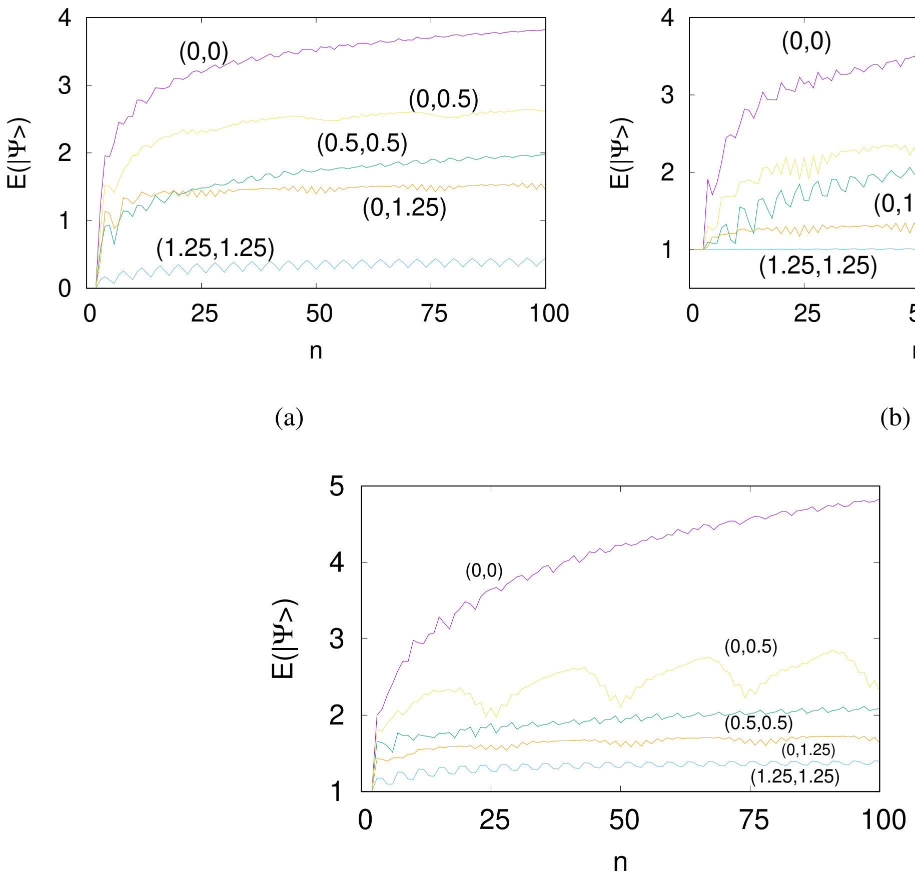


(a)

(b)

(c)

FIG. 5. Variation of bi-partite entanglement $E(|\psi\rangle)$ against dimension less time $n$ (step number) for two pi-phase interacting walkers starting from : (a) $|Sep\rangle$ state, (b) $|\psi^{+}\rangle$ state, (c) $|\psi^{-}\rangle$ state. In each figure, different curves have been drawn for different $(\alpha_1, \alpha_2)$ combinations as shown inside the figures.

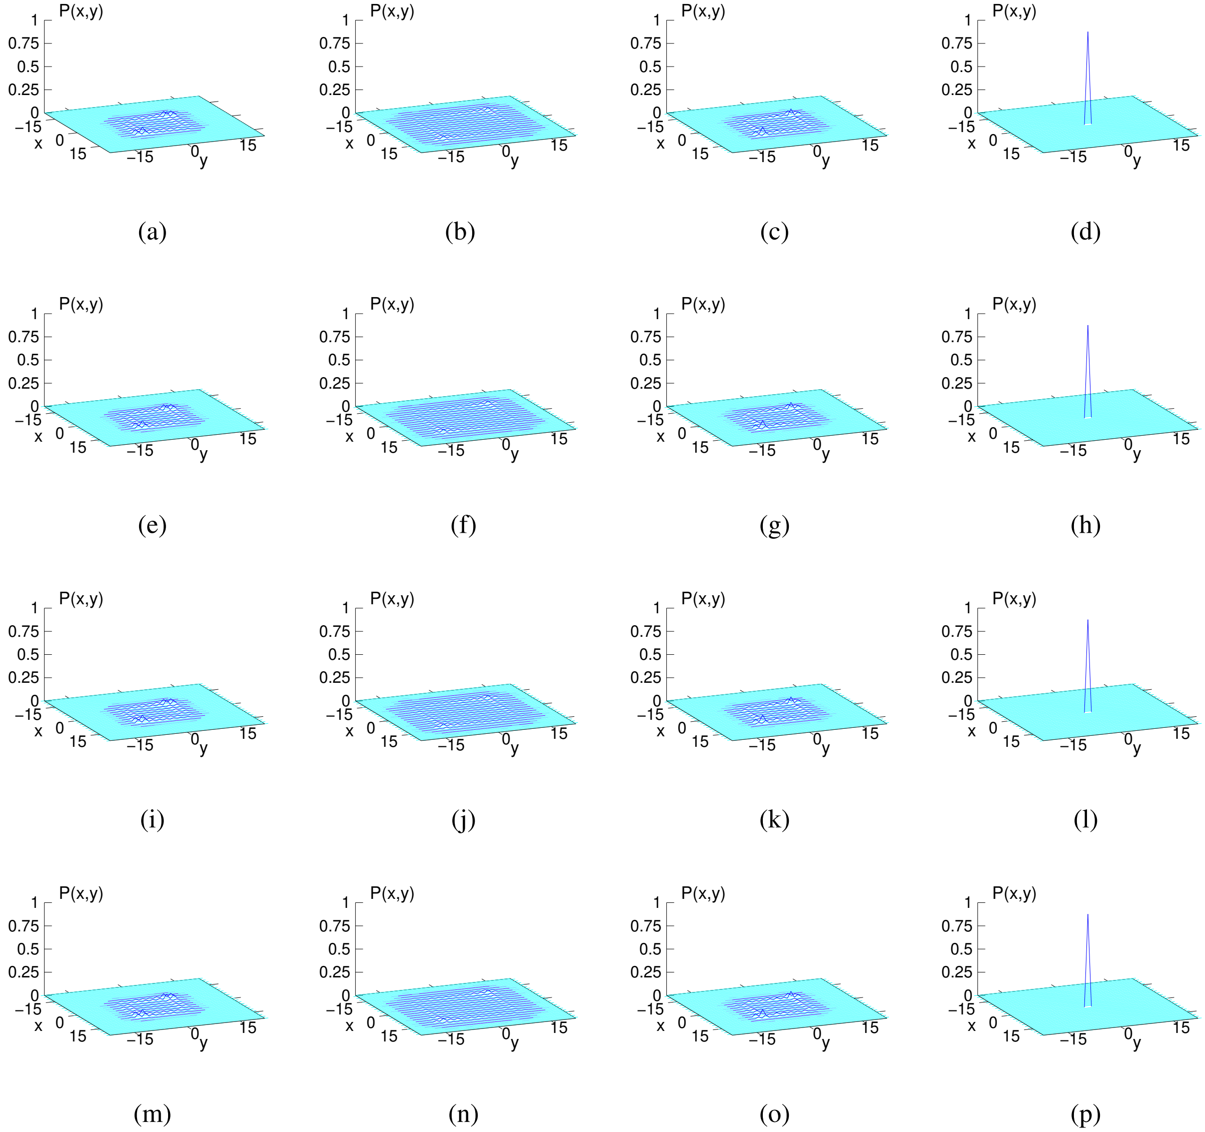


FIG. 6. Here figures (a)-(p) show two-particle probability distributions $P(x, y)$ for two $\mathbb{1}$ interacting walkers starting from $|\psi^+\rangle$ initial state under the influence of the time-dependent coin $\hat{C}_{\Phi,\Phi}$ ($q = 1, p = 50$) after completion of the following different time steps : (a) $n = 12$, (b) $n = 25$, (c) $n = 37$, (d) $n = 50$, (e) $n = 62$, (f) $n = 75$, (g) $n = 87$, (h) $n = 100$, (i) $n = 112$, (j) $n = 125$, (k) $n = 137$, (l) $n = 150$, (m) $n = 162$, (n) $n = 175$, (o) $n = 187$, (p) $n = 200$ ( $n$ is the dimensionless time (step number)). The points for which $P(x, y) > 0.00001$, are colored in blue. The plots clearly show that the structure of $P(x, y)$ changes with time in a periodic manner with a time period of 50 steps as the elements of the sets {(a),(e),(i),(m)}; {(b),(f),(j),(n)}; {(c),(g),(k),(o)} and {(d),(h),(l),(p)} exhibit identical structures of $P(x, y)$ among themselves.

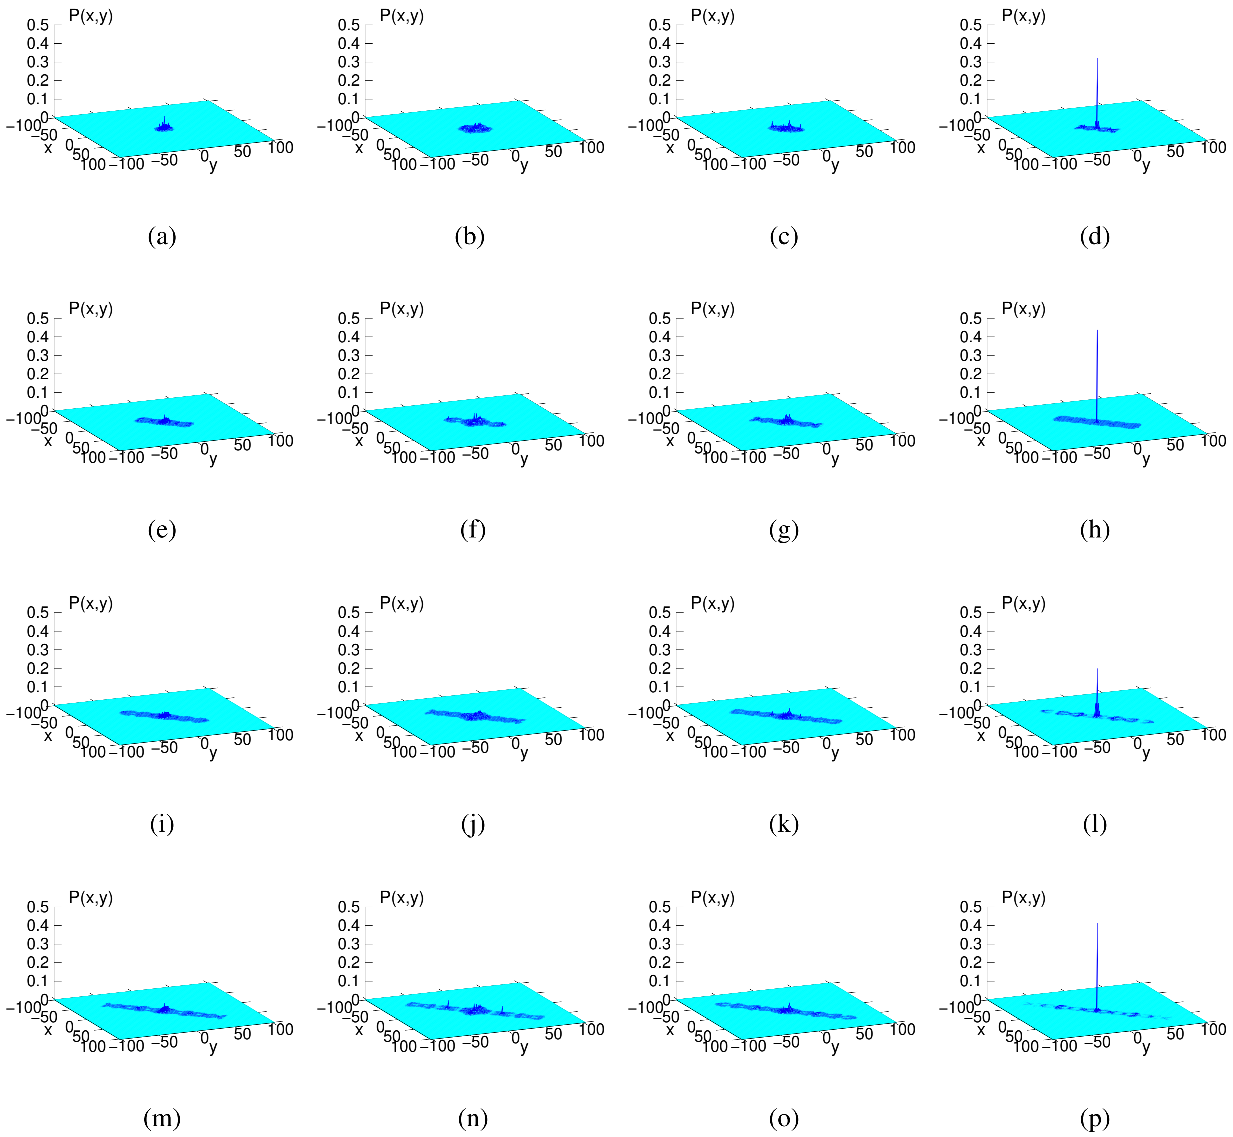


FIG. 7. Here figures (a)-(p) show two-particle probability distributions $P(x, y)$ for two $\pi$-phase interacting walkers starting from $|\psi^+\rangle$ initial state under the influence of the time-dependent coin $\hat{C}_{\Phi,\Phi}$ $(q = 1, p = 50)$ after completion of the following different time steps : (a) $n = 12$, (b) $n = 25$, (c) $n = 37$, (d) $n = 50$, (e) $n = 62$, (f) $n = 75$, (g) $n = 87$, (h) $n = 100$, (i) $n = 112$, (j) $n = 125$, (k) $n = 137$, (l) $n = 150$, (m) $n = 162$, (n) $n = 175$, (o) $n = 187$, (p) $n = 200$ ( $n$ is the dimensionless time (step number)). The points for which $P(x, y) > 0.00001$, are colored in blue. The plots clearly show that the structure of $P(x, y)$ does not change with time in a periodic manner.

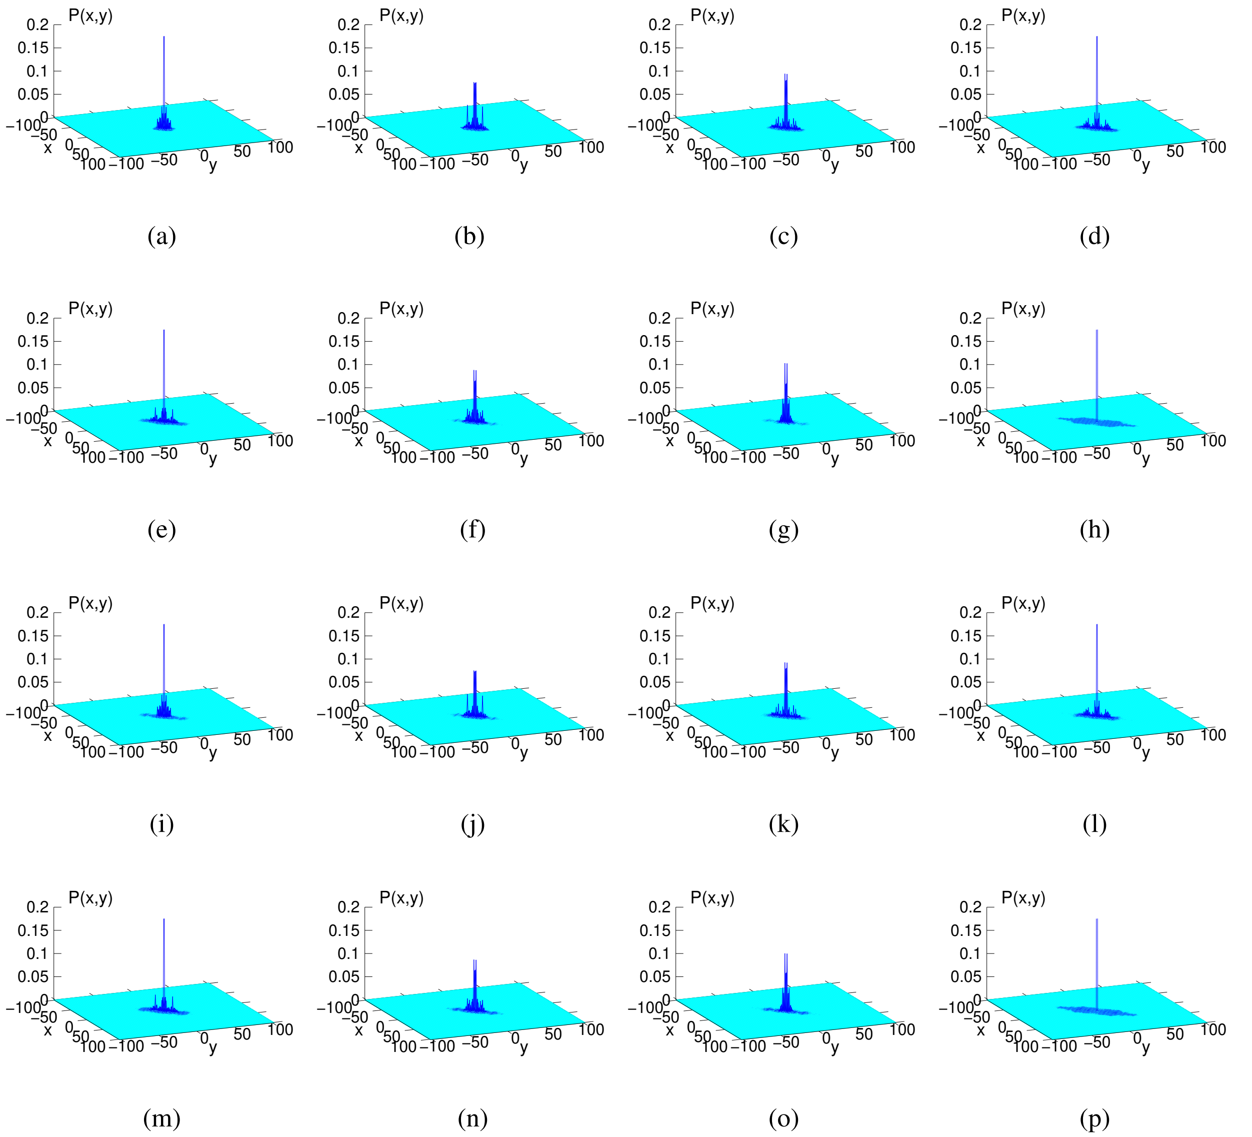


FIG. 8. Here figures (a)-(p) show two-particle probability distributions $P(x, y)$ for two $\pi$-phase interacting walkers starting from $|\psi^+\rangle$ initial state under the influence of the time-dependent coin $\hat{C}_{\Phi,\Phi}$ $(q = 4, p = 50)$ after completion of the following different time steps : (a) $n = 12$, (b) $n = 25$, (c) $n = 37$, (d) $n = 50$, (e) $n = 62$, (f) $n = 75$, (g) $n = 87$, (h) $n = 100$, (i) $n = 112$, (j) $n = 125$, (k) $n = 137$, (l) $n = 150$, (m) $n = 162$, (n) $n = 175$, (o) $n = 187$, (p) $n = 200$ ( $n$ is the dimensionless time (step number)). The points for which $P(x, y) > 0.00001$, are colored in blue. The plots clearly show that the structure of $P(x, y)$ changes with time in a periodic manner with a time period of 100 steps. The difference between Fig. 7 and Fig. 8 is the choice of coin parameters. In Fig. 7, there was no dynamic localization but here, we see dynamic localization.

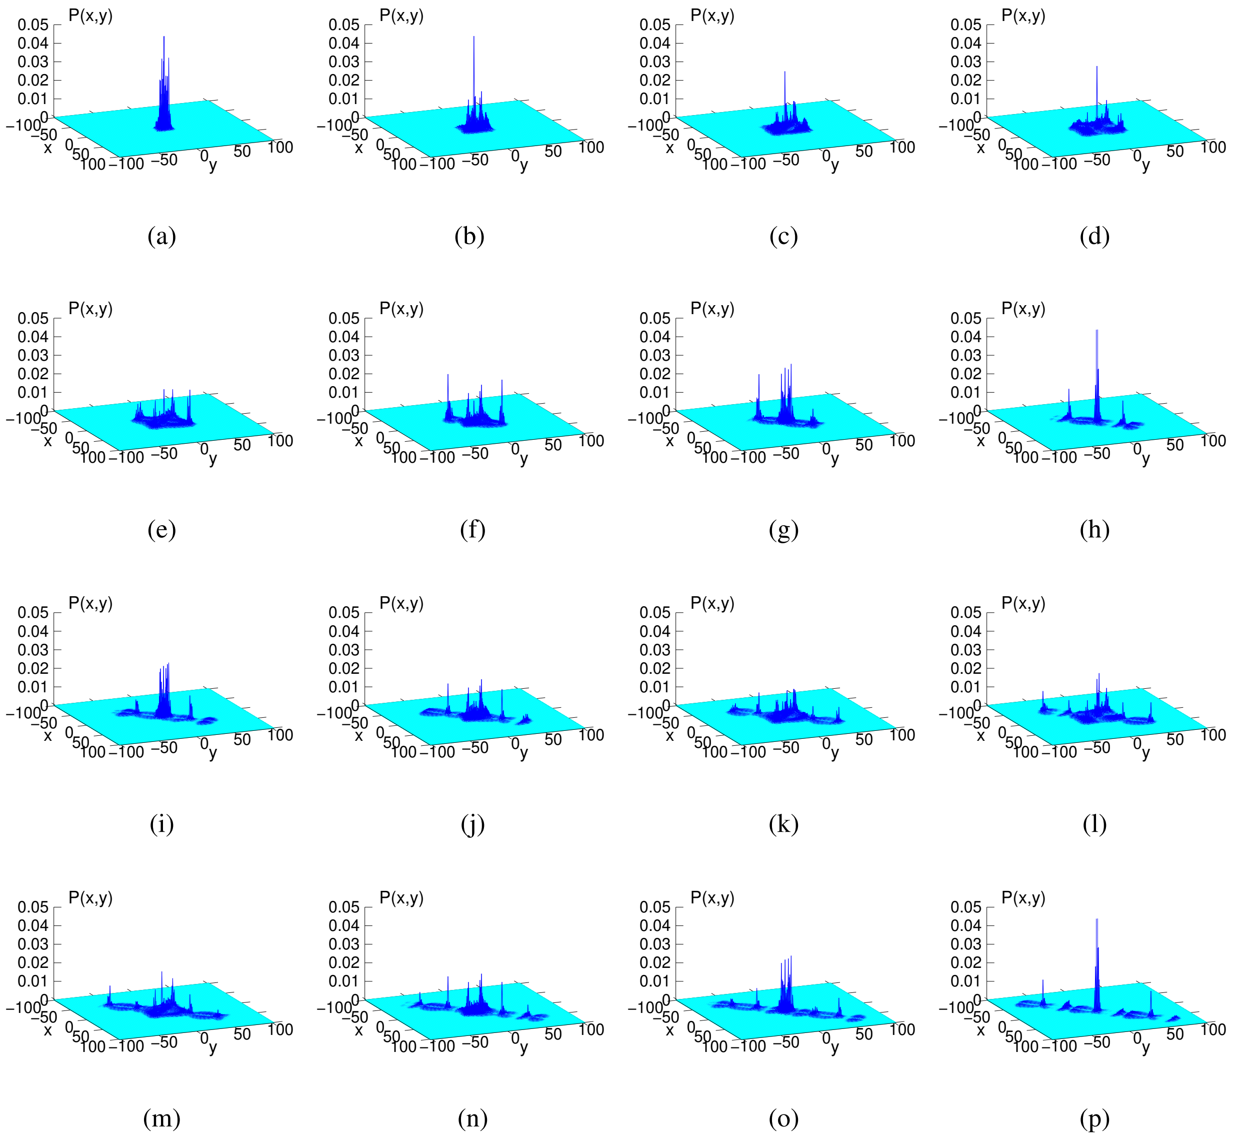


FIG. 9. Here figures (a)-(p) show two-particle probability distributions $P(x,y)$ for two $\pi$-phase interacting walkers starting from $|Sep\rangle$ initial state under the influence of the time-dependent coin $\hat{C}_{\Phi,\Phi}$ $(q = 1, p = 100)$ after completion of the following different time steps : (a) $n$ = 12, (b) $n$ = 25, (c) $n$ = 37, (d) $n$ = 50, (e) $n$ = 62, (f) $n$ = 75, (g) $n$ = 87, (h) $n$ = 100, (i) $n$ = 112, (j) $n$ = 125, (k) $n$ = 137, (l) $n$ = 150, (m) $n$ = 162, (n) $n$ = 175, (o) $n$ = 187, (p) $n$ = 200 ( $n$ is the dimensionless time (step number)). The points for which $P(x,y) > 0.00001$, are colored in blue. The plots clearly show that the structure of $P(x,y)$ does not change with time in a periodic manner.
